# Supplementary material for: Finite-time Polytropic Steering Reveals Non-monotonic Irreversibility
Source: arXiv:2602.13765 source file (2026-10-21)
Supplement: Supplementary file 1 [file SM.pdf]

# Supplemental Materials

This document is devoted to providing the detailed derivations and for supporting discussions to the main text. The contents of the Supplemental Materials are listed as follows

## Contents


**1 The detailed derivation for polytropic steering of underdamped Brownian particles 2**
1.1 The effective temperature evolution and polytropic protocols . . . 2
1.2 Thermodynamic quantities and the irreversible entropy generation . . . 2

**2 The stochastic framework for polytropic steering of overdamped Brownian particles 3**
2.1 Langevin dynamics . . . 3
2.2 The effective temperature evolution and polytropic protocols . . . 3
2.3 Thermodynamic quantities and the irreversible entropy generation . . . 4

**3 The asymptotic scaling analysis of irreversible entropy generation 4**
3.1 The adiabatic limit . . . 5
3.2 The isothermal limit . . . 5

**4 The role of the initial temperature offset $\delta$ 5**

**5 Simulation details 6**
5.1 The numerical Solution of the Control Protocol . . . 6
5.2 Langevin Dynamics Simulation . . . 7
5.3 The calculation of thermodynamic quantities . . . 7
5.4 The convergence and Robustness Verification . . . 7

**6 The polytropic steering of the ideal gas system 7**
6.1 The finite-time polytropic process . . . 8
6.2 The qualification of irreversibility . . . 9
6.3 The application in thermodynamic cycles . . . 9

# 1 The detailed derivation for polytropic steering of underdamped Brownian particles

In this section, we provide detailed derivation for the polytropic steering of a Brownian particle in the underdamped limit discussed in the main text.

## 1.1 The effective temperature evolution and polytropic protocols

By leveraging the Fokker–Planck equation corresponding to the Eq. (2) from the main text, we can derive a Maxwell–Boltzmann distribution. Through this distribution correspondence, a rigorous definition of the effective temperature $\theta(t) = 2\langle E(t)\rangle / f_n$ can be established. Subsequently, based on the first law of thermodynamics, the time-dependent evolution function for the particle's effective temperature can be deduced as

$$\dot{\theta}(t) = \frac{\dot{\lambda}(t)}{\lambda(t)}\theta(t) - \Gamma_n \left[\theta(t) - T_{\mathrm{s}}\right]. \tag{S1}$$

We now impose the polytropic constraint, defined by the relation $\theta\lambda^{\xi} = \text{const.}$, where $\xi$ is the polytropic index and const. is a constant determined by the initial conditions $(k_0, \theta_0)$. Time differentiation of this constraint yields $\dot{\lambda}/\lambda = -\dot{\theta}/(\xi\theta)$. Substituting this relation into the dynamical equation (S1), we obtain

$$\dot{\theta}(t) = -\frac{\dot{\theta}(t)}{\xi} - \Gamma_n \left[\theta(t) - T_{\mathrm{s}}\right]. \tag{S2}$$

With the initial condition $\theta|_{t=0} \equiv \theta_0 = (1+\delta)\, T_{\mathrm{s}}$ ($\delta \neq 0$, $\delta < 0$ for expansion, $\delta > 0$ for compression), the above differential equation (S2) is solved as

$$\theta = \theta(t) = \delta T_{\mathrm{s}} \exp\left(-\frac{\xi\Gamma_n}{\xi+1}t\right) + T_{\mathrm{s}}, \tag{S3}$$

and correspondingly, the work parameter change during the polytropic process $\theta(t)\lambda^{\xi}(t) = \theta_0\lambda_0^{\xi}$ follows as

$$\lambda(t) = \lambda_0 \left[\frac{\delta}{1+\delta}\exp\left(-\frac{\xi\Gamma_n}{\xi+1}t\right) + \frac{1}{1+\delta}\right]^{-\frac{1}{\xi}} \tag{S4}$$

with $\lambda_0$ is the initial work parameter of the particle. For the case where $\lambda_{\mathrm{f}}/\lambda_0 \equiv u$ ($\lambda_{\mathrm{f}} = \lambda(\tau)$) is given, where $u$ is the compression ratio of the process, the relation between the normalized process duration $\tilde{\tau} \equiv \tau/\tau_{\mathrm{r}}$ and the polytropic index can be derived from Eq. (S4) as

$$\tilde{\tau} = -\frac{1+\xi}{\xi}\ln\left[\frac{(1+\delta)\, u^{-\xi} - 1}{\delta}\right]. \tag{S5}$$

Eqs. (S4) and (S5) serve as practical operational protocols to realize the given $\xi$ polytropic process.

## 1.2 Thermodynamic quantities and the irreversible entropy generation

The ensemble average of internal energy for the underdamped Brownian particle can be expressed as $\langle E\rangle = f_n\theta(t)/2$. The increment of trajectory ensemble average work for this system is

$$\langle dW\rangle = \frac{f_n}{2}\theta_0\lambda_0^{\xi}\lambda^{-\xi-1}d\lambda. \tag{S6}$$

Integrate from initial $(k_0, \theta_0)$ to final $(k_f, \theta_f)$ states, we have

$$W = \frac{f_n(1+\delta)T_{\mathrm{s}}}{2\xi}\left[1 - u^{-\xi}\right]. \tag{S7}$$

Using the first law of thermodynamics we have the heat as

$$Q = \frac{f_n(1+\delta)T_{\mathrm{s}}}{2}\left(\frac{\xi+1}{\xi}\right)\left[u^{-\xi} - 1\right]. \tag{S8}$$

Finally, we evaluate the irreversible entropy generation (IEG), which in this regime arises from the heat flux between the system at effective temperature $\theta$ and the reservoir at $T_s$. The corresponding IEG rate reads $\dot{S}_{\rm ir} = \dot{Q}/\theta - \dot{Q}/T_s$. Utilizing the energy balance $\dot{Q} = \dot{E} - \dot{W}$, the cumulative IEG over a duration $\tau$ is given by

$$\Delta S_{\rm ir} = \int_0^\tau (\frac{\dot{E} - \dot{W}}{\theta} - \frac{\dot{E} - \dot{W}}{T_s})dt. \tag{S9}$$

By substituting the polytropic trajectories and the control equation (S4), the analytical expression for IEG is simplified to

$$\Delta S_{\rm ir} = (\xi + 1)\left[\xi^{-1}(1+\delta)(1-u^{-\xi}) - \ln u\right], \tag{S10}$$

where $u = k_f/k_0$ is the compression/expansion ratio. This result recovers the universal scaling behavior discussed in the main text, confirming that the thermodynamic cost of polytropic steering is preserved in the underdamped regime.

# 2 The stochastic framework for polytropic steering of overdamped Brownian particles

In this section, we establish a stochastic derivation for the polytropic steering of a Brownian particle in the overdamped limit. This framework provides the theoretical basis for the control protocols and thermodynamic quantities discussed in the main text.

## 2.1 Langevin dynamics

We consider a one-dimensional overdamped Brownian particle confined within a time-dependent harmonic potential $U(x, k_t) = k_t x^2/2$ for simplicity and without loss of generality. The governing Langevin equation in the overdamped limit is given by

$$\gamma\dot{x} = -\frac{k_t}{m}x + \frac{\zeta(t)}{m}, \tag{S11}$$

where $\gamma$ denotes the friction coefficient. To ensure the consistency of the steady-state distribution with the Boltzmann factor $P_{\rm eq}(x) \propto e^{-U/T_s}$, the stochastic force $\zeta(t)$ must satisfy the fluctuation-dissipation theorem

$$\langle\zeta(t)\zeta(t')\rangle = 2m\gamma T_s\,\delta(t-t'), \tag{S12}$$

where $T_s$ is the temperature of the heat reservoir. By representing the white noise as a Wiener increment, $\xi(t)\,dt = \sqrt{2m\gamma T_s}\,dW_t$, Eq. (S11) can be recast into the Ito stochastic differential equation

$$dx = -\frac{k_t}{m\gamma}x\,dt + \sqrt{\frac{2T_s}{m\gamma}}\,dW_t. \tag{S13}$$

To track the energetic evolution of the system, we define the instantaneous energy as $E(t) = U(x(t), t) = \frac{1}{2}k_t\,x(t)^2$. According to Ito's lemma, the differential of a scalar function $f(x,t)$ is expressed as

$$df = \partial_t f\ dt + \partial_x f\ dx + \frac{1}{2}\partial_{xx} f\ (dx)^2. \tag{S14}$$

By substituting the specific form of the harmonic potential into Eq. (S14) and utilizing the property $(dW_t)^2 = dt$, the stochastic increment of the system energy is derived as

$$dE = \left(\frac{1}{2}\dot{k}_t x^2 - \frac{k_t^2}{m\gamma}x^2 + \frac{k_t T_s}{m\gamma}\right)dt + k_t x\sqrt{\frac{2T_s}{m\gamma}}dW_t. \tag{S15}$$

## 2.2 The effective temperature evolution and polytropic protocols

Following the framework of stochastic thermodynamics, the ensemble-averaged energy $\langle E\rangle$ can be associated with an effective temperature $\theta(t)$ via the relation $\langle E\rangle = \frac{1}{2}\theta(t)$ [1]. Taking the expectation of Eq. (S15) and noting that the expectation of the Wiener term vanishes, we obtain the dynamical equation for $\theta(t)$

$$\dot{\theta} = \frac{\dot{k}_t}{k_t}\theta - \frac{2k_t}{m\gamma}(\theta - T_s). \tag{S16}$$

Equation (S16) describes the thermal relaxation of the particle towards the reservoir temperature $T_s$, modulated by the active variation of the trap stiffness $k_t$.

We now impose the polytropic constraint, defined by the relation $\theta k_t^{\xi} = \text{const.}$, where $\xi$ is the polytropic index and const. is a constant determined by the initial conditions $(k_0, \theta_0)$. Time differentiation of this constraint yields $\dot{k}_t/k_t = -\dot{\theta}/(\xi\theta)$. Substituting this relation into the dynamical equation (S16) yields the steering protocol for the trap stiffness

$$\frac{\dot{k}_t}{k_t} = \frac{2k_t}{m\gamma(\xi+1)}\left[1 - \frac{1}{1+\delta}\left(\frac{k_t}{k_0}\right)^{\xi}\right], \tag{S17}$$

where $\delta = (\theta_0 - T_s)/T_s$ characterizes the initial thermal deviation from the reservoir.

### 2.3 Thermodynamic quantities and the irreversible entropy generation

The average work rate is defined by the variation of the potential parameters, $\langle \dot{W} \rangle = \frac{1}{2}\langle x^2 \rangle \dot{k}_t$. With the relation $\langle x^2 \rangle = \theta/k_t$, the total work performed during a process from $k_0$ to $k_f$ is integrated as

$$W = \frac{\theta_0}{2\xi}\left[1 - \left(\frac{k_0}{k_f}\right)^{\xi}\right] \tag{S18}$$

Applying the first law of thermodynamics, $\Delta E = W + Q$, where $\Delta E = (\theta_f - \theta_0)/2$, the heat exchanged with the reservoir is obtained as

$$Q = \frac{\theta_0}{2}\left(\frac{\xi+1}{\xi}\right)\left[\left(\frac{k_0}{k_f}\right)^{\xi} - 1\right]. \tag{S19}$$

Finally, we evaluate the irreversible entropy generation (IEG), which in this regime arises from the heat flux between the system at effective temperature $\theta$ and the reservoir at $T_s$. The corresponding IEG rate reads $\dot{S}_{\text{ir}} = \dot{Q}/\theta - \dot{Q}/T_s$ [2]. Utilizing the energy balance $\dot{Q} = \dot{E} - \dot{W}$, the cumulative IEG over a duration $\tau$ is given by

$$\Delta S_{\text{ir}} = \int_0^{\tau} \left(\frac{\dot{E} - \dot{W}}{\theta} - \frac{\dot{E} - \dot{W}}{T_s}\right) dt. \tag{S20}$$

By substituting the polytropic trajectories and the control equation (S17), the analytical expression for IEG is simplified to

$$\Delta S_{\text{ir}} = \frac{1}{2}(\xi+1)\left[\xi^{-1}(1+\delta)(1-u^{-\xi}) - \ln u\right], \tag{S21}$$

where $u = k_f/k_0$ is the compression/expansion ratio. This result recovers the universal scaling behavior discussed in the main text, confirming that the thermodynamic cost of polytropic steering is preserved in the overdamped regime.

## 3 The asymptotic scaling analysis of irreversible entropy generation

As discussed in the main text, the irreversible entropy generation (IEG) exhibits a non-monotonic dependence on the process duration $\tilde{\tau}$, characterized by a transition from linear growth in the fast-driving regime to a $1/\tilde{\tau}$ decay in the quasi-static limit. To rigorously elucidate the mathematical origin of these scaling laws, this section provides an asymptotic analysis of the IEG near the two fundamental thermodynamic boundaries: the adiabatic limit ($\xi \to -1$) and the isothermal limit ($\xi \to 0$).

The IEG for a system of underdamped Brownian particles in the Section 1 reads

$$\Delta S_{\text{ir}} = (\xi+1)\left[\xi^{-1}(1+\delta)(1-u^{-\xi}) - \ln u\right], \tag{S22}$$

together with the corresponding the $\tau - \xi$ relation

$$\tilde{\tau} = -(1+\xi^{-1})\ln\left[(1+\delta^{-1})u^{-\xi} - \delta^{-1}\right]. \tag{S23}$$

Taylor expansions of Eqs. (S22) and (S23) around $\xi = 0$ and $\xi = -1$ yield the analytical coefficients that govern dissipation in the adiabatic and isothermal regimes, respectively.

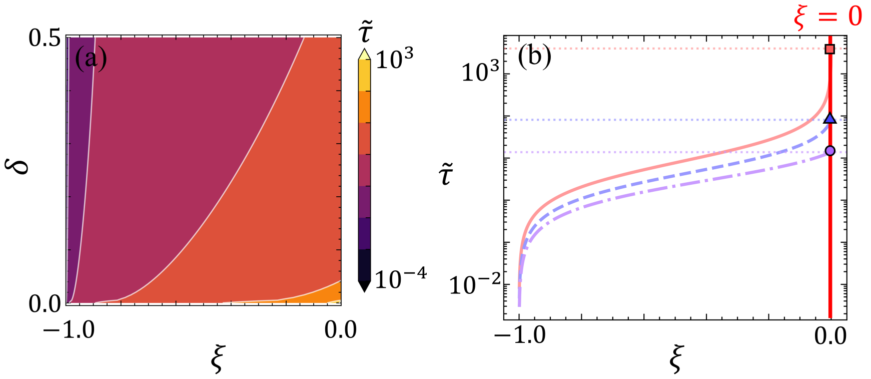


**Fig. S1** The influence of initial temperature offset $\delta$ on the duration, and $u = 1.5$ is used in this figure. (a) The heatmap of the normalized process duration $\tilde{\tau}$ as functions of $\xi$ and $\delta$. (b) $\tilde{\tau}$ versus $\xi$ for three different $\delta = 10^{-4}$ (pink solid curve), $5 \times 10^{-3}$ (blue dashed curve), and $3 \times 10^{-2}$ (purple dash-dotted curve). The maximum process durations $\tilde{\tau}_{\max}$ corresponding to $\xi = 0$ are marked with the pink square, blue triangle, and purple circle.

### 3.1 The adiabatic limit

For adiabatic regime, $\tilde{\tau}$ can be expressed as

$$\tilde{\tau} \approx A_{-1}\,(\xi + 1)\,. \tag{S24}$$

Additionally, the Taylor expression of $\Delta S_{\rm ir}$ at $\xi = -1$ denotes as

$$\Delta S_{\rm ir} \approx B_{-1}\,(\xi + 1)\,. \tag{S25}$$

Finally, we can obtain

$$\Delta S_{\rm ir} \approx \kappa_1(\delta, u)\tilde{\tau} = \frac{B_{-1}}{A_{-1}}\tau, \tag{S26}$$

where

$$A_{-1} = \ln\left[\frac{(1+\delta)u - 1}{\delta}\right], \quad B_{-1} = (1+\delta)(u-1) - \ln u.$$

### 3.2 The isothermal limit

For isothermal regime, the expansion approximation of $\tilde{\tau}$ can be expressed as

$$\frac{1}{\tilde{\tau}} \approx A_0 + B_0\xi. \tag{S27}$$

Additionally, we can obtain

$$\Delta S_{\rm ir} \approx C_0 + D_0\xi. \tag{S28}$$

Finally, we have

$$\Delta \tilde{S}_{\rm ir} \approx \kappa_2(\delta, u)/\tilde{\tau} + \kappa_0(\delta, u) = \frac{D_0}{B_0}\frac{1}{\tilde{\tau}} + C_0 - \frac{A_0 D_0}{B_0}, \tag{S29}$$

where

$$A_0 = \frac{\delta}{(1+\delta)\ln u}, \; B_0 = -\frac{\ln u + 2\delta}{2(1+\delta)\ln u}, \; C_0 = \delta \ln u, \; D_0 = \delta\ln u - \frac{1}{2}(1+\delta)\ln^2 u.$$

## 4 The role of the initial temperature offset $\delta$

As noted in the main text, the realization of a finite-time polytropic process is contingent upon a non-zero initial temperature offset $\delta \equiv \theta_0/T_s - 1$. This section demonstrates the mathematical necessity of this non-equilibrium starting point and examines how the $\delta$ dictate $\tilde{\tau}$ and IEG.

The governing equation for the finite-time polytropic process reveals a mathematical singularity when $\delta = 0$. Physically, this implies that if a system begins in perfect equilibrium with the reservoir, a quasi-static polytropic path with a specific index $\xi$ (other than the isothermal or isochoric limits) cannot be uniquely initiated without an infinitesimal heat flow to select the trajectory. However, we demonstrate that the limit $\delta \to 0$ is well-behaved, as shown in Figs. S1 and S2. For any arbitrarily small but finite perturbation, the

control protocol remains robust and experimentally accessible (very rapid quenching from the equilibrium state).

As illustrated in Fig. S1, the limit $\xi = 0$ corresponds to an endoreversible isothermal process. For a given initial temperature offset $\delta$, the process duration is characterized by a finite timescale that diverges only as $\delta \to 0$, thereby recovering the conventional quasi-static limit. This behavior is further corroborated by the entropy analysis in Fig. S2, which reveals that a perfectly reversible isothermal transformation is attainable only in the limit of vanishing $\delta$. The existence of an initial temperature gradient inherently induces an irreversible entropy flux and the asymptotic points provided in the isothermal limit confirm this dissipation mechanism arising from initial thermal mismatch.

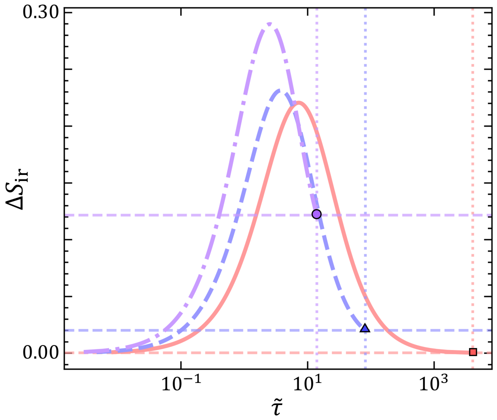


**Fig. S2** $\Delta S_{\rm ir}$ versus $\tilde{\tau}$ for three different $\delta = 10^{-4}$ (pink solid curve), $5 \times 10^{-3}$ (blue dashed curve), and $3 \times 10^{-2}$ (purple dash-dotted curve). The theoretical isothermal limits are given by dotted line. The maximum process durations $\tilde{\tau}_{\rm max}$ corresponding to $\xi = 0$ are marked with the pink square, blue triangle, and purple circle.

# 5 Simulation details

In this section, we provide an in-depth description on how all our numerical simulations are implemented. To validate the theoretical predictions of the polytropic process for an overdamped Brownian particle, we performed numerical simulations of the stochastic Langevin dynamics. The simulation framework consists of three coupled parts: (i) the numerical solution of the control protocol $k_t$, (ii) the ensemble simulation of particle trajectories, and (iii) a rigorous convergence verification.

## 5.1 The numerical Solution of the Control Protocol

The time evolution of the trap stiffness $k_t$, required to maintain the polytropic condition $\theta k^{\xi} = \text{const.}$, is governed by the nonlinear ordinary differential equation (ODE) derived in the main text,

$$\frac{\dot{k}_t}{k_t} = \frac{2k_t}{m\gamma(\xi+1)}\left[1 - \frac{1}{1+\delta}\left(\frac{k_t}{k_0}\right)^{\xi}\right]. \tag{S30}$$

We solved this initial value problem using the *scipy.integrate.solve_ivp* package in Python.

**Algorithm Selection**: To ensure numerical stability particularly when the polytropic index $\xi$ approaches the singular value of $-1$, we implemented an adaptive solver strategy:

- For general cases, we utilized the explicit Runge-Kutta method of order 5(4) (RK45).
- For cases where $\xi \approx -1$ (specifically $|\xi + 1| < 10^{-2}$), the dynamics become stiff. Here, we switched to the Backward Differentiation Formula (BDF) method.
- To prevent numerical division errors, a regularization parameter $\epsilon = 10^{-12}$ was applied to the denominator term $(\xi + 1)$.

**Event Detection**: The duration of the protocol $\tau$ was determined dynamically. We employed a root-finding event detection algorithm to identify the precise time instant $t = \tau$ at which the stiffness reached the target compression value $k(\tau) = k_{\rm final}$.

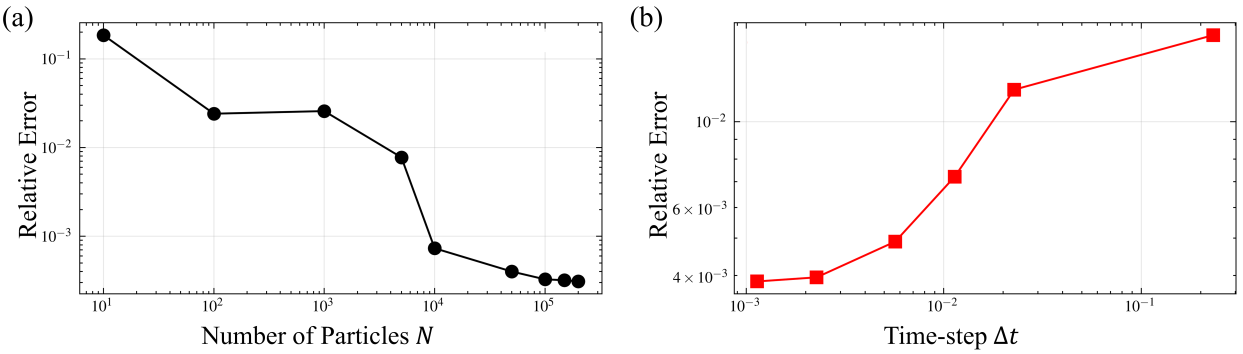


**Fig. S3** Relative Error of work as a function of (a) ensemble size $N$ and (b) time-step $\Delta t$.

## 5.2 Langevin Dynamics Simulation

**Discretization Scheme**: We simulated the trajectories of an ensemble of $N = 10^6$ non-interacting particles using the Euler-Maruyama scheme. The iterative update rule for the position $x_n$ of the $n$-th particle at time step $j$ is given by

$$x_n\left(t_{j+1}\right) = x_n\left(t_j\right) - \frac{k\left(t_j\right)}{\gamma} x_n\left(t_j\right)\Delta t + \sqrt{\frac{2T_s\Delta t}{\gamma}}\mathcal{N}(0,1), \tag{S31}$$

where $\Delta t$ is the time step. The initial positions $\{x_n(0)\}$ were sampled from the equilibrium Boltzmann distribution $P(x,0) \propto \exp(-U/\theta_0)$.

## 5.3 The calculation of thermodynamic quantities

Thermodynamic observables were computed via ensemble averaging over the $N$ simulated trajectories.

- Effective Temperature: $\theta_{\text{sim}} = k(t)\left\langle x^2(t)\right\rangle \approx \frac{k(t)}{N}\sum_{n=1}^{N} x_n^2(t)$.

- Stochastic Work: To ensure numerical accuracy, we employed the midpoint approximation for the position term in the discretized work $dW = \frac{1}{2}x^2 dk$ as

$$W(t) = \sum_{j=0}^{M(t)} \frac{1}{2}\left[\frac{x_n^2\left(t_j\right) + x_n^2\left(t_{j+1}\right)}{2}\right]\left(k\left(t_{j+1}\right) - k\left(t_j\right)\right), \tag{S32}$$

  where $M(t)$ denote the time discretization of total steps.

- Heat $Q$ was derived using $Q(t) = \Delta U(t) - W(t)$, where $\Delta U(t) = \frac{1}{2}k(t)x^2(t) - \frac{1}{2}k_0 x^2(0)$.

## 5.4 The convergence and Robustness Verification

To ensure the reliability of the numerical results, we conducted comprehensive convergence tests

- Ensemble Size Convergence ($N$): increasing $N$ from $10^1$ to $10^5$ reduces the relative error compared to the analytical solution to below 0.1%.

- Time-step Convergence ($\Delta t$): The discretization error of the Euler-Maruyama scheme was monitored by varying $\Delta t$. We ensured that $\Delta t$ is significantly smaller than the instantaneous relaxation time $\tau_r = \gamma/k(t)$ throughout the protocol. A convergence of the error with respect to $\Delta t$ was observed.

# 6 The polytropic steering of the ideal gas system

In the main text, we established a finite-time polytropic steering framework for Brownian particles, focusing on the interplay between stochastic energetics and time-dependent confinement. To demonstrate the broader universality of this paradigm, we now extend the polytropic steering principle to a macroscopic classical system–the ideal gas. The objective of this section is to show that the protocols derived for microscopic stochastic systems are not mere artifacts of the harmonic potential or specific noise realizations. Instead,

they represent a fundamental class of thermodynamic transformations that can be generalized to any system where the evolution of internal energy follows a consistent linear structure.

## 6.1 The finite-time polytropic process

The concept of a polytropic process $pV^{\xi} = \text{const.}$, where $p$ and $V$ denote the pressure and the volume, is a cornerstone of textbook equilibrium thermodynamics, typically introduced as a heuristic interpolation between the idealized isothermal and adiabatic limits. However, in its conventional form, the polytropic paradigm remains a purely phenomenological description of state-space trajectories, lacking a macroscopic kinetic foundation for operations performed in finite time. To bridge this gap, we consider a dynamic model of an ideal gas where the finite-time heat exchange with the environment is explicitly accounted for.

The system is thermally isolated from the external environment and comprises an ideal gas with temperature $T$ driven by a heat reservoir with constant temperature $T_{\mathrm{s}}$. When the gas is compressed or expanded by a piston, the energy conservation ($\dot{U} = \dot{Q} + \dot{W}$) law reads

$$C_V \dot{T} = -\kappa (T - T_{\mathrm{s}}) - p\dot{V}. \tag{S33}$$

Here, $C_V$ represents the heat capacity of an ideal gas at constant volume, and the heat transfer is assumed to follow Newton's law of cooling with the coefficient $\kappa$. Note that $\tau_{\mathrm{r}} = C_V/\kappa$ is the characteristic time for the gas to thermalize in the reservoir, which is much larger than the internal relaxation time $t_{\mathrm{in}}$ of the gas [2]. The polytropic process equation can be written in terms of $T$ and $V$ as $TV^{\xi-1} = \text{constant}$, differentiating which with respect to time yields

$$\dot{T}V + (\xi - 1)T\dot{V} = 0. \tag{S34}$$

From Eq. (S33), eliminating $p$ with the ideal gas state equation $pV = NT$ and further eliminating $V$ and $\dot{V}$ with Eq. (S34), we obtain

$$C_V \dot{T} = -\kappa (T - T_{\mathrm{s}}) + N\frac{\dot{T}}{\xi - 1}, \tag{S35}$$

where $N$ is the gas particle number. With the initial condition $T|_{t=0} \equiv T_0 = (1+\delta)\,T_{\mathrm{e}}$ ($\delta \neq 0$, $\delta < 0$ for expansion, and $\delta > 0$ for compression), the above differential equation is solved as

$$T = T(t) = \delta T_{\mathrm{s}} \exp\left[\frac{\kappa(\gamma - 1)(\xi - 1)}{N(\gamma - \xi)}t\right] + T_{\mathrm{s}}, \tag{S36}$$

and correspondingly, the volume change during the polytropic process $T(t)[V(t)]^{(\xi-1)} = T_0 V_0^{(\xi-1)}$ follows as

$$V(t) = V_0 \left\{\frac{\delta}{1+\delta} \exp\left[\frac{\kappa(\gamma - 1)(\xi - 1)}{N(\gamma - \xi)}t\right] + \frac{1}{1+\delta}\right\}^{\frac{1}{1-\xi}}, \tag{S37}$$

where $V_0$ is the initial volume of the gas.

For the case where $V_{\mathrm{f}}/V_0 \equiv u$ ($V_{\mathrm{f}} = V(\tau)$) is given, where $u$ is the compression ratio of the process, the relation between the normalized process duration $\tilde{\tau} \equiv \tau/t_{\mathrm{r}}$ and the polytropic index can be derived from Eq. (S37) as

$$\tilde{\tau} = \frac{\gamma - \xi}{\xi - 1} \ln\left[\frac{(1+\delta)\,u^{1-\xi} - 1}{\delta}\right]. \tag{S38}$$

Eqs. (S37) and (S38) serve as practical operation protocols to realize the given $\xi$ polytropic process.

It is highly instructive to note that the resulting protocols for the ideal gas [Eqs. (S37)-(S38)] are formally identical to those derived for the underdamped Brownian particle in the main text. This mathematical isomorphism is not coincidental but stems from the fact that both systems, despite their vastly different scales and noise characteristics, share a common governing structure for their temperature (or average energy) evolution. Consequently, the polytropic paradigm can be naturally translated from the stochastic realm to classical engineering systems via a simple mapping of physical parameters-such as substituting the trap stiffness control with piston volume modulation. This unity reinforces the role of the polytropic index as a universal control knob for finite-time thermodynamics.

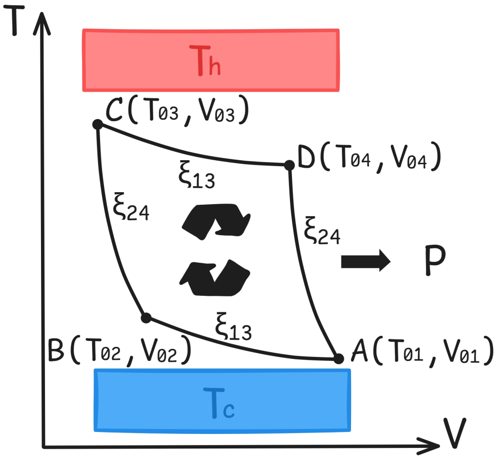


**Fig. S4** The schematic T-V diagram of a four strokes polytropic cycle. The processes C→B (polytropic index $\xi_{24}$) and B→A ($\xi_{13}$) release heat to the low-temperature reservoir at $T_c$, while A→D ($\xi_{24}$) and D→C ($\xi_{13}$) absorb heat from the high-temperature reservoir at $T_h$. The cycle outputs net work.

## 6.2 The qualification of irreversibility

For the ideal gas undergoing the polytropic process of interest, IEG is only attributed to the heat flow resulting from the discrepancy of temperature between the system and the heat reservoir [3], namely, $\Delta S_{\mathrm{ir}} = \int_0^\tau (\dot{Q}/T - \dot{Q}/T_{\mathrm{e}})dt$, which is specifically obtained as

$$\Delta \tilde{S}_{\mathrm{ir}} = \frac{\gamma - \xi}{\gamma - 1}\left(1 + \frac{\delta + 1}{\xi - 1}\frac{u^{1-\xi} - 1}{\ln u}\right). \tag{S39}$$

Here, we have used $\dot{Q} = C_\xi \dot{T}$ with the polytropic heat capacity $C_\xi = C_V(\xi - \gamma)(\xi - 1)$, $\Delta\tilde{S}_{\mathrm{ir}} \equiv \Delta S_{\mathrm{ir}}/\Delta S_{\mathrm{iso}}$, and $\Delta S_{\mathrm{iso}} = N \ln u$ denotes the reversible entropy change in a quasi-static isothermal process of $\xi = 1$. Substituting Eq. (S38) into the above equation, IEG as a function of process duration is straightforward determined.

## 6.3 The application in thermodynamic cycles

We present a general polytropic cycle of heat engines, as shown in Fig. S4. The closed conditions of the cycle are

$$\begin{aligned} T_{01}V_{01}^{\xi_{13}-1} &= T_{02}V_{02}^{\xi_{13}-1}, \\ T_{02}V_{02}^{\xi_{24}-1} &= T_{03}V_{03}^{\xi_{24}-1}, \\ T_{03}V_{03}^{\xi_{13}-1} &= T_{04}V_{04}^{\xi_{13}-1}, \\ T_{04}V_{04}^{\xi_{24}-1} &= T_{01}V_{01}^{\xi_{24}-1}. \end{aligned} \tag{S40}$$

Since the heat capacity of a polytropic process depends only on the polytropic index, the heat absorbed or released in each process can be straightforwardly calculated based on the parameters of A, B, C, and D as follows

$$\begin{aligned} Q_{A\to B} &= C_V \frac{\xi_{13} - \gamma}{\xi_{13} - 1}(T_{02} - T_{01}), \\ Q_{B\to C} &= C_V \frac{\xi_{24} - \gamma}{\xi_{24} - 1}(T_{03} - T_{02}), \\ Q_{C\to D} &= C_V \frac{\xi_{13} - \gamma}{\xi_{13} - 1}(T_{04} - T_{03}), \\ Q_{D\to A} &= C_V \frac{\xi_{24} - \gamma}{\xi_{24} - 1}(T_{01} - T_{04}). \end{aligned} \tag{S41}$$

With Eqs. (S40) and (S41), we can obtain the simplified expressions of efficiency and work output of the cycle as

$$
\begin{aligned}
W &= Q_{A\to B} + Q_{B\to C} + Q_{C\to D} + Q_{D\to A} \\
&= C_V \left[T_{01}\left(\mu^{\xi_{13}-1}-1\right) + T_{03}\left(\mu^{1-\xi_{13}}-1\right)\right]\left(\frac{\xi_{13}-\gamma}{\xi_{13}-1} - \frac{\xi_{24}-\gamma}{\xi_{24}-1}\right).
\end{aligned} \tag{S42}
$$

Here, using $Q_{\mathrm{a}}$ and $Q_{\mathrm{r}}$ to denote the heat absorbed and released respectively, we have

$$
\begin{aligned}
Q_{\mathrm{a}} = \frac{1}{2}\{&[1+\mathrm{sgn}(\mathrm{Q_{A\to B}})]\,Q_{A\to B} + [1+\mathrm{sgn}(\mathrm{Q_{B\to C}})]\,Q_{B\to C} \\
&+ [1+\mathrm{sgn}(\mathrm{Q_{C\to D}})]\,Q_{C\to D} + [1+\mathrm{sgn}(\mathrm{Q_{D\to A}})]\,Q_{D\to A}\},
\end{aligned} \tag{S43}
$$

where

$$
\mathrm{sgn(x)} = \begin{cases} -1, & x \le 0 \\ 1, & x > 0. \end{cases}
$$

For specific situation $Q_{\mathrm{a}} = Q_{C\to D} + Q_{D\to A}$, we have

$$
\begin{aligned}
\eta &= \frac{W}{Q_{\mathrm{a}}} = \frac{W}{Q_{C\to D}+Q_{D\to A}} \\
&= \frac{\left(2-\mu^{\xi_{13}-1}-\mu^{1-\xi_{13}}\right) + \left(1-T_{01}/T_{03}\right)\left(\mu^{\xi_{13}-1}-1\right)}{1-\mu^{1-\xi_{13}} + \left(1-T_{01}/T_{03}\right)\frac{(\xi_{24}-\gamma)(\xi_{13}-1)}{(\gamma-1)(\xi_{13}-\xi_{24})}},
\end{aligned} \tag{S44}
$$

where $\mu \equiv V_{01}/V_{02} = V_{04}/V_{03}$.

For some particular polytropic index, this efficiency formula can be degenerated into the familiar form. When $\xi_{13}=1$, $\xi_{24}=\gamma$, $T_{01}=T_{\mathrm{c}}$ and $T_{03}=T_{\mathrm{h}}$, Eq. (S44) is reduced to

$$
\begin{aligned}
\eta &= \frac{\eta_{\mathrm{C}}\left(\mu^{\xi_{13}-1}-1\right)}{1-\mu^{1-\xi_{13}}} \\
&= \frac{\eta_{\mathrm{C}}\left[e^{(\xi_{13}-1)\ln\mu}-1\right]}{1-e^{(1-\xi_{13})\ln\mu}} \\
&\approx \frac{\eta_{\mathrm{C}}\left(\xi_{13}-1\right)\ln\mu}{\left(\xi_{13}-1\right)\ln\mu} = \eta_{\mathrm{C}},
\end{aligned} \tag{S45}
$$

which is back to the result of the Carnot cycle. When $\xi_{13}=0$, $\xi_{24}=\gamma$, $T_{01}=T_{\mathrm{c}}$ and $T_{03}=T_{\mathrm{h}}$, Eq. (S44) is reduced to

$$
\begin{aligned}
\eta &= \frac{\left(2-\mu^{-1}-\mu\right)+\eta_{\mathrm{C}}\left(\mu^{-1}-1\right)}{1-\mu} \\
&= 1-\mu^{-1}\left(1-\eta_{\mathrm{C}}\right),
\end{aligned} \tag{S46}
$$

which is back to the result of the Ranking cycle.

To investigate the specific performance of the cycle, we set the symmetric polytropic index $\xi$, thereby circumventing the complexity while capturing the basic characteristics arising from fast driving protocol. As illustrated in Fig. S5(a), we propose a thermodynamic cycle, termed the polytropic-adiabatic cycle (PAC), which consists of two symmetric polytropic processes with same $\xi$ and two adiabatic processes. The geometric feature of PAC is solely characterized by $\xi$. As $\xi \to 1$, PAC converges to endoreversible Carnot cycle; while when $\xi \to \gamma$, the polytropic and adiabatic processes degenerate, resulting in the cycle disappearing. Note that the cycle duration is entirely contributed by the polytropic processes according to Eq. (S38), such that the efficiency and power of the cycle are explicitly determined by $\xi$. The trade-off relation between power and efficiency is obtained by varying $\xi$, as shown in Fig. S5(b). Each local point on this trade-off is plotted with a certain $\xi$, the value of which is visualized by the color map.

The power-efficiency trade-off relation of PAC exhibits consistent behavior with the $1/\tau$-scaling. Namely, as $\xi$ decreases (approaching the blue zone of the gradient curve), the cycle efficiency approaches the Carnot limit but at the cost of zero power output. Notably, the EMP of PAC surpasses the upper bound predicted by the Low-Dissipation (LD) model. While similar behavior has been observed in micro quantum systems,

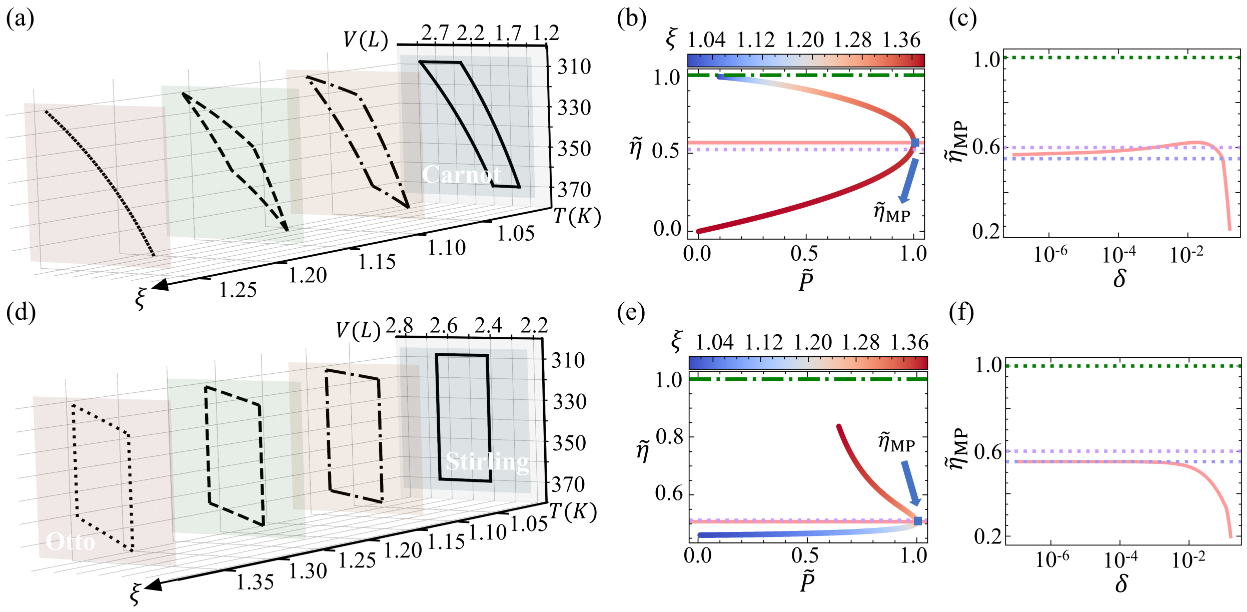


**Fig. S5** (a) The transition of the T-V diagram from the endoreversible Carnot cycle to the degenerate of polytropic and adiabatic process with the high- and low-temperature reservoirs set at 369.8 $(K)$ and 308.2 $(K)$, respectively, and a compression ratio of 1.1. (b) Normalized efficiency $\tilde{\eta}$ versus normalized power $\tilde{P}$ trade-off. The dash-dotted green line (upper) shows the Carnot efficiency $\eta_{\mathrm{C}} = 9.1 \times 10^{-2}$, and the EMP of polytropic-adiabatic cycle is highlighted using blue square and pink solid curve. EMP of Low-Dissipation model is given by a purple dotted line. $\xi$ of the cycle is shown with a color map on the trade-off curve. (c) EMP of PAC (solid pink curve) as the function of $\delta$, and the Carnot efficiency, the upper bound of low-dissipation model and CA efficiency are represented as green dotted, purple dotted and blue dotted line, respectively. (d) The transition from the Stirling cycle to the Otto cycle with the high- and low-temperature reservoirs set at 369.8 $(K)$ and 308.2 $(K)$, respectively, and a compression ratio of 1.05. (e) The trade-off between normalized power and normalized efficiency. (f) EMP of polytropic-isochoric (solid curve) as the function of $\delta$, and the Carnot efficiency, the upper bound of LD model and CA efficiency are plotted by green dotted, purple dotted and blue dotted line, respectively.

where phase transitions originate from collective advantages and many-body interactions [4–6], our ideal gas system lacks internal interactions. Consequently, we examine the relation between EMP and $\delta$, as shown in Fig. S5(c). The results indicate that EMP exhibits a nonmonotonic behavior: as $\delta$ approaches 0, it converges to the result predicted by the CA model $\eta_{\mathrm{CA}} = 1 - \sqrt{1 - \eta_{\mathrm{C}}}$; subsequently, it surpasses the result of the LD model in certain intermediate regions; and finally, it monotonically decreases to 0 as $\delta$ further increases.

The Stirling and Otto cycles are practical thermodynamic cycles widely used in engineering applications [7]. By combining polytropic and isochoric processes, we propose a polytropic-isochoric cycle (PIC), which enables a continuous transition from the Stirling cycle ($\xi \to 1$) to the Otto cycle ($\xi \to \gamma$) as illustrated in Fig. S5(d). Notably, the time for the isochoric branch must be included in the total cycle time, and both satisfy Eq. (S38). For the isochoric process, this equation corresponds to $\xi \to \infty$. Increasing $\xi$ has two primary effects: i) it directly reduces the time of the polytropic branch, and ii) it shifts the intersection between the polytropic and isochoric processes upward, thereby reducing the isochoric process time. Overall, the performance of the PIC is solely determined by $\xi$.

The power-efficiency trade-off relation is depicted in Fig. S5(e), illustrating its behavior during varying $\xi$. In addition to distinct shapes with PAC, the gradient curves of PIC exhibit reversed colors. Specifically, the power-efficiency trade-off relation of PIC scales with $\tau$: as $\xi$ increases (approaching the red zone of the gradient curve), the cycle efficiency improves correspondingly. This difference arises from the presence of isochoric branches in PIC, which increase IEG compared to the adiabatic branches. The isochoric branches contribute more significantly to the IEG than the polytropic process, owing to their efficient heat exchange and longer thermal relaxation times with the reservoirs. Higher value of $\xi$ can reduce the ratio of isochoric process in PIC, resulting in low dissipation thus higher efficiency. Because of the greater role of the isochoric process in IEG, $\delta$ (a key parameter for the polytropic branches) in PIC serves only as an upper bound for the quasi-static cycle efficiency. This differs from its role in PAC, where $\delta$ balances power and efficiency at the point of EMP. This distinction also explains why the EMP in PIC varies monotonically with $\delta$, as shown in Fig. S5(f).

## References


[1] Y.H. Chen, J.F. Chen, Z. Fei, H.T. Quan, Microscopic theory of the Curzon-Ahlborn heat engine based on a Brownian particle. Phys. Rev. E **106**(2), 024105 (2022). https://doi.org/10.1103/PhysRevE.106.024105

[2] Y.H. Ma, R.X. Zhai, J. Chen, C.P. Sun, H. Dong, Experimental Test of the 1 / $\tau$ -Scaling Entropy Generation in Finite-Time Thermodynamics. Phys. Rev. Lett. **125**(21), 210601 (2020). https://doi.org/10.1103/PhysRevLett.125.210601

[3] U. Seifert, Stochastic thermodynamics, fluctuation theorems and molecular machines. Rep. Prog. Phys. **75**(12), 126001 (2012). https://doi.org/10.1088/0034-4885/75/12/126001

[4] N. Golubeva, A. Imparato, Efficiency at Maximum Power of Interacting Molecular Machines. Phys. Rev. Lett. **109**(19), 190602 (2012). https://doi.org/10.1103/PhysRevLett.109.190602

[5] M.L. Bera, S. Julià-Farré, M. Lewenstein, M.N. Bera, Quantum heat engines with Carnot efficiency at maximum power. Phys. Rev. Res. **4**(1), 013157 (2022). https://doi.org/10.1103/PhysRevResearch.4.013157

[6] S. Liang, Y.H. Ma, D.M. Busiello, P. De Los Rios, Minimal Model for Carnot Efficiency at Maximum Power. Phys. Rev. Lett. **134**(2), 027101 (2025). https://doi.org/10.1103/PhysRevLett.134.027101

[7] D. Dai, Z. Liu, R. Long, F. Yuan, W. Liu, An irreversible Stirling cycle with temperature difference both in non-isothermal and isochoric processes. Energy **186**, 115875 (2019). https://doi.org/10.1016/j.energy.2019.115875
